# Supplementary material for: Verification and the Risk of a Wrong Cascade
Source: arXiv:2508.20538 ancillary file (2026-11-29)
Supplement: Supplementary file 1 [file FalseCascades_slide.pdf]

# False Cascades and the Cost of Truth

Georgy Lukyanov    Darina Cheredina

# Roadmap

- Motivation
  - Cascades vs. truth with decentralized checks
- Model in one slide
- Binary benchmark
  - Cutoff & a simple breakability test
- Continuous actions
  - responsiveness vs. coarsening
- Resilience frontier & quick welfare takeaways
- Related literature
- Conclusion & Q&A

# Why verification matters in cascades

- Actions are public
- Signals are private  $\Rightarrow$  herding/cascades
- Occasional **verification** can create **public proof**
- Question: when do decentralized checks **break** false cascades?
- Aim
  - Clean conditions
  - Minimal primitives
  - Transparent thresholds

# Setup

- Binary state
- Agents act sequentially
- Observe public history
- Private binary signal, precision  $q > 1/2$
- Option
  - Investigate at cost  $c$
  - Success  $p$  only if the claim is true
- If proof arrives: verifiable, disclosed
  - Baseline:  $V \geq 0$
- Actions
  - Binary benchmark
  - Continuous with conformity  $\rightarrow$  later

# Investigation is a cutoff in the posterior

- Single crossing  $\Rightarrow$  unique cutoff  $x^*$ .
- Rule: investigate iff posterior

$$x \geq x^*$$

- Location vs. classical cascade bands

$$\mu \in [0, 1 - q] \cup [q, 1]$$

- Selection: ties favor investigation & disclosure
  - Robust to small trembles

# Breakability at the boundary: a simple test

- Consider a **wrong** boundary cascade
  - Belief at  $1 - q$  or  $q$
- Decentralized proof breaks the cascade with positive probability when

$$\frac{c}{V} \leq p$$

- Intuition
  - “cheap enough” checks  $\Rightarrow$  someone reveals  $\Rightarrow$  beliefs reset
- Comparative statics
  - $\uparrow p$  or  $\downarrow c/V \Rightarrow$  easier to break

# Tiny numeric example

- Fix  $q = 0.6$ ,  $V = 1$ ,  $c = 0.20$ .
- If  $p \geq 0.20$ : boundary false cascades are **breakable**.
- If  $p < 0.20$ : decentralized proof too rare
  - Consequently, there is **persistence at the boundary**

# Responsiveness threshold under coarsening

- Best response

$$a^* = \gamma x + (1 - \gamma)\mu$$

- Public sees coarsened actions (grid step  $h$ ).
- Soft-channel informativeness requires:

$$\gamma \Delta x(\mu, q) \geq h$$

- Below threshold
  - Actions stop separating
  - Disclosures carry the load
- Design levers
  - $\uparrow \gamma$  (responsiveness)
  - $\downarrow h$  (finer observation)



# A tractable frontier

- Breakable set in  $(p, c/V)$  is  $\uparrow$  in  $p$ ,  $\downarrow$  in  $c/V$
- With continuous actions:
  - Expands with  $\uparrow \gamma$  and  $\downarrow h$
- Diagnostic
  - Where to expect self-correction vs. persistence

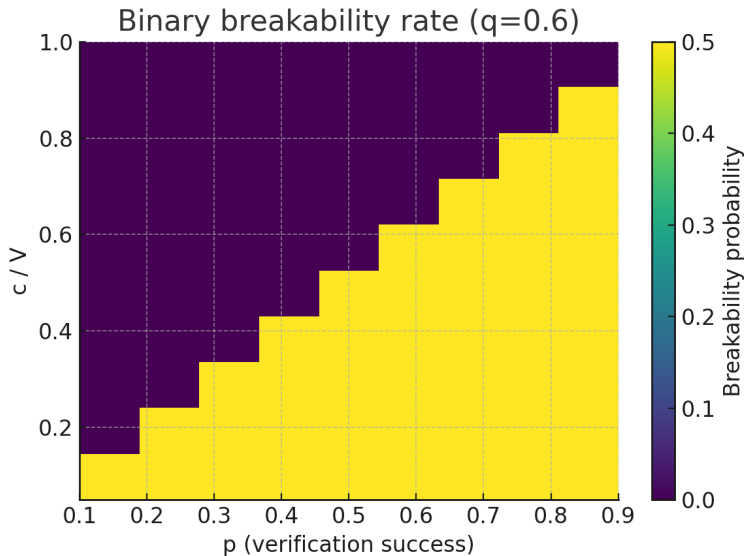

# Welfare takeaways

- Small  $\uparrow p$  or small  $\downarrow c/V$  can flip persistence to breakability.
- In high-conformity/coarse settings
  - Proofs substitute for muted actions
- Targeted subsidies or platform tools that boost  $p$  are high leverage

# Related literature

- Cascades
  - Banerjee; Bikhchandani–Hirshleifer–Welch
- Learning speed/geometry
  - Arieli; Hann–Caruthers–Martynov–Tamuz
- Verifiable disclosure
  - Grossman–Milgrom; Bertomeu–Cianciaruso
- Conformity/coarsening
  - Bernheim; Xu

# Takeaway

- Simple boundary logic for breaking false cascades via proof
- Clear threshold when soft actions go mute under coarsening
- Frontier guides policy:  $\uparrow p, \downarrow c/V, \uparrow \gamma, \downarrow h$

# Thanks!

## Q&A
